# Supplementary material for: LVP-M3: Language-aware Visual Prompt for Multilingual Multimodal Machine Translation
Source: arXiv:2210.15461 source file (2022-11-28)
Supplement: Supplementary file 1 [file appendix.tex]

% % This must be in the first 5 lines to tell arXiv to use pdfLaTeX, which is strongly recommended.
% \pdfoutput=1
% % In particular, the hyperref package requires pdfLaTeX in order to break URLs across lines.

% \documentclass[11pt]{article}

% % Remove the "review" option to generate the final version.
% \usepackage[review]{acl}

% % Standard package includes
% \usepackage{times}
% \usepackage{latexsym}

% % For proper rendering and hyphenation of words containing Latin characters (including in bib files)
% \usepackage[T1]{fontenc}
% % For Vietnamese characters
% % \usepackage[T5]{fontenc}
% % See https://www.latex-project.org/help/documentation/encguide.pdf for other character sets

% % This assumes your files are encoded as UTF8
% \usepackage[utf8]{inputenc}

% % This is not strictly necessary, and may be commented out,
% % but it will improve the layout of the manuscript,
% % and will typically save some space.
% \usepackage{microtype}

% % If the title and author information does not fit in the area allocated, uncomment the following
% %
% %\setlength\titlebox{<dim>}
% %
% % and set <dim> to something 5cm or larger.

% % custom packages
% %\usepackage{subcaption}
% \usepackage{graphicx}
% \usepackage{booktabs}
% \usepackage{multicol}
% \usepackage{multirow}
% \usepackage{amsmath}
% \usepackage{amssymb}
% \usepackage{bbding}
% \usepackage{subfigure}


% \newcommand{\SmallEquation}{\fontsize{8.5pt}{\baselineskip}\selectfont}
% \newcommand{\MiddleEquation}{\fontsize{9pt}{\baselineskip}\selectfont}
% \newcommand{\BigEquation}{\fontsize{9.5pt}{\baselineskip}\selectfont}
% \newcommand{\ourmethod}{\textsc{mlTrans}}
% \title{Supplementary Material for \ourmethod{}}

% % Author information can be set in various styles:
% % For several authors from the same institution:
% % \author{Author 1 \and ... \and Author n \\
% %         Address line \\ ... \\ Address line}
% % if the names do not fit well on one line use
% %         Author 1 \\ {\bf Author 2} \\ ... \\ {\bf Author n} \\
% % For authors from different institutions:
% % \author{Author 1 \\ Address line \\  ... \\ Address line
% %         \And  ... \And
% %         Author n \\ Address line \\ ... \\ Address line}
% % To start a seperate ``row'' of authors use \AND, as in
% % \author{Author 1 \\ Address line \\  ... \\ Address line
% %         \AND
% %         Author 2 \\ Address line \\ ... \\ Address line \And
% %         Author 3 \\ Address line \\ ... \\ Address line}

% \author{
% }

% % \begin{document}
% % \maketitle
% \appendix


% % \vspace{-100mm}
% \begin{table*}[!htp]
% \centering
% %\resizebox{0.75\textwidth}{!}{
% \resizebox{0.9\textwidth}{!}{
% \begin{tabular}{l|cccccc|c}
% \toprule
% Model (X$\rightarrow$En)   & Fr & Cs & De & Lv & Hi & Tr & Avg$_{all}$ \\
% \midrule
% \multicolumn{8}{c}{\textit{Text-only Multilingual MT Systems}} \\ 
% \midrule
%   Text Transformer \cite{english-centered}   & 46.6 & 36.9 & 39.1 & 44.5 & 48.6 & 45.6 & 43.6 \\
% \midrule
% 	\multicolumn{8}{c}{\textit{Multilingual MMT Systems}} \\
% \midrule

%   Vision Matters (Gated fusion) \cite{vision_matters}  & 51.3 & 40.0 & 41.9 & 48.7  & 52.8 & 48.4 & 47.1 \\
%   Vision Matters (Concatenation) \cite{vision_matters}  &46.2   & 36.5 & 38.8  & 44.2 & 48.2 & 45.5 & 43.2 \\
%   \ourmethod{} (w/o LVPG)  & 51.0 & 39.7 & 41.6  & 48.5 & 52.4 & 48.0 & 46.9\\
%   \ourmethod{}  & \bf 52.1 & \bf 40.8  & \bf 42.2 & \bf 49.0 & \bf 53.3 & \bf 49.1 & \bf 47.8  \\
% \bottomrule
% \end{tabular}}
% \caption{BLEU scores of X$\rightarrow$En tasks on M$^{3}$-Multi30K test set.}
% \label{table:xenmulti30k}
% % \vspace{-5pt}
% \end{table*}

% \begin{table*}[!htp]
% \centering
% %\resizebox{0.75\textwidth}{!}{
% \resizebox{0.9\textwidth}{!}{
% \begin{tabular}{l|cccccc|c}
% \toprule
% Model (X$\rightarrow$En)   & Fr & Cs & De & Lv & Hi & Tr & Avg$_{all}$ \\
% \midrule
% \multicolumn{8}{c}{\textit{Text-only Multilingual MT Systems}} \\ 
% \midrule
%   Text Transformer \cite{english-centered}   &53.6  & 48.1 & 51.2 & 47.0 & 49.5 & 41.8 & 48.5 \\
% \midrule
% 	\multicolumn{8}{c}{\textit{Multilingual MMT Systems}} \\
% \midrule

%   Vision Matters (Gated fusion) \cite{vision_matters}  & 54.3 & 49.9 & 52.3 & 47.6 & 50.0 & 42.3 & 49.4 \\
%   Vision Matters (Concatenation) \cite{vision_matters}  &53.2  & 47.7 & 50.0 & 46.7 & 48.9 & 41.3 & 48.1 \\
%   \ourmethod{} (w/o LVPG)  & 53.9 & 49.0 & 51.7 & 47.3 & 49.7 & 42.0 & 48.9 \\
%   \ourmethod{}  & \bf 58.1 & \bf 51.3  & \bf 55.6 & \bf 49.1 & \bf 52.6 & \bf 43.2 & \bf 51.7  \\
% \bottomrule
% \end{tabular}}
% \caption{BLEU scores of X$\rightarrow$En tasks on M$^{3}$-AmbigCaps test set.}
% \label{table:xenamcaps}
% % \vspace{-5pt}
% \end{table*}

% \section{More Results}
% % \subsection{More Results}
% As shown in Table \ref{table:xenmulti30k} and Table \ref{table:xenamcaps},
% we also report the translation results of different methods by translating six languages into English (i.e., X$\rightarrow$En) on two datasets.
% we observe our \ourmethod{} still outperforms other baseline methods a lot,
% which further demonstrates the effectiveness of our newly proposed \ourmethod{} method for Multilingual MMT.




% \section{Related Work}
% How to fully utilize the multimodal context plays an important role for Multimodal Machine Translation (MMT). The recent commonly-used MMT methods can be divided into three categories.
% (1) Using global visual features directly. 
% For instance, ~\citet{huang2016attention} proposed to concatenate global and regional visual features with source sequences, and~\citet{calixto2017incorporating} used global visual features as additional tokens in the source sequence. 
% (2) Exploiting visual features via attention scheme.
% For example,
% ~\citet{libovicky2017attention} tried to explore flat and hierarchical combinations for fusing the attention-based contexts from two modalities.
% ~\citet{calixto2017doubly} introduced the visual features into the MMT model by using an independent attention module. 
% ~\citet{helcl2018cuni} adopted the timestep-specific source-side context vector as attention query to dynamically produce the visual context features. 
% (3) Combining other vision tasks with translation task by multitask learning. 
% For example, 
% ~\cite{elliott2017imagination} decomposed multimodal translation into two sub-tasks (i.e., translation and visual grounding). 
% ~\cite{calixto2019latent} applied a continuous latent variable by including the underlying semantic information extracted from texts and images. 
% ~\cite{yin2020novel}  adopted a unified multi-modal graph to obtain semantic relationships between different modalities.
% In contrast to existing works,
% we focus on the Multilingual MMT using one single model.
% \noindent\textbf{Multilingual Language Models}. 
% Pretrained multilingual Transformer-based language models (e.g., mBERT~\cite{kenton2019bert}
%  and XLM-R~\cite{conneau2020unsupervised}) utilize the same pretraining strategies as their respective monolingual counterparts (e.g., BERT~\cite{kenton2019bert} and RoBERTa~\cite{liu2019roberta}).
% They are pretrained via self-supervised masked language
% modelling objective (MLM) on concatenated
% text corpora of more than 100 languages.
% ~\cite{artetxe2020cross} proposed a method to transfer monolingual representations to new languages in an unsupervised fashion and provide new insights on the generalization abilities of multilingual models.
% ~\cite{hu2020xtreme} introduced the 
% Cross-lingual TRansfer Evaluation of Multilingual Encoders 
% (XTREME) benchmark to evaluate the
% cross-lingual generalization capabilities,
% ~\cite{karthikeyan2019cross} also provide a comprehensive study of the contribution of different components in M-BERT to its cross-lingual ability.~\cite{rust2021good} show that monolingually adapted tokenizers can robustly improve monolingual performance
% of multilingual models.
% Overall, when compared with these methods, we focus on the multilingual setting for MMT,
% which has not been investigated before.



% \bibliography{custom}
% \bibliographystyle{acl_natbib}
% \end{document}
